# Supplementary material for: Dispersion Analysis of Finite Difference and Discontinuous Galerkin Schemes for Maxwell's Equations in Linear Lorentz Media
Source: arXiv:1810.01723 source file (2018-10-03)
Supplement: Supplementary file 1 [file appendix.tex]

\section{Analysis of $\omega(k)$}

First we define new notations
\begin{align}
\displaystyle \label{Nota}
\WH{k}:= kh, \qquad
\WH{\omega} := \frac{\omega}{\omega_1}, \qquad
\WH{\gamma} := \frac{\gamma}{\omega_1}, \qquad
\end{align}

\noindent where $\WH{k}$ and $\WH{\omega}$ are dimensionless. From the exact dispersion relation \eqref{DisEx4}, we have
\begin{align}
\displaystyle
\left( \frac{\WH{k}}{\omega_1h} \right)^2
&= \WH{\omega}^2
\left[
\epsilon_\infty 
- \frac{\epsilon_d}{\WH{\omega}^2 + 2i\,\WH{\gamma}\,\WH{\omega} - 1}
\right]. 
\end{align}

\noindent Using the fact that $\epsilon_d = \epsilon_s - \epsilon_\infty$, we get
\begin{align}
\displaystyle
\left( \frac{\WH{k}}{\omega_1h} \right)^2\left[
\WH{\omega}^2 + 2i\,\WH{\gamma}\,\WH{\omega} - 1
\right]
&=
\epsilon_\infty \WH{\omega}^4 + 2\epsilon_\infty i \,\WH{\gamma}\, \WH{\omega}^3
- \epsilon_s \WH{\omega}^2.
\end{align}

\noindent Thus, we simplify the above equation to obtain 
\begin{align}
\displaystyle
\WH{\omega}^4 + 2i\,\WH{\gamma}\,\WH{\omega}^3 
- \frac{1}{\epsilon_\infty}
\left(
\epsilon_s +  \frac{\WH{k}^2}{(\omega_1h)^2} 
\right) \WH{\omega}^2
- \frac{2i}{\epsilon_\infty} \WH{\gamma}\, \frac{\WH{k}^2}{(\omega_1h)^2} \, \WH{\omega}
+ \frac{1}{\epsilon_\infty}\frac{\WH{k}^2}{(\omega_1h)^2}  = 0. \label{qq6}
\end{align}

\noindent To analyze the root of equation \eqref{qq6}, we first introduce the following notations
\begin{subequations}\label{Not1}
	\begin{align}
	\displaystyle  
	P(x) &:= -\frac{1}{\epsilon_\infty}\left(\epsilon_s + \frac{x^2}{(\omega_1h)^2}  \right)
	+ \frac{3}{2}\WH{\gamma}^2,  \\ 
	R(x) &:= -i\,\WH{\gamma}\,\left[
	\WH{\gamma}^2 -\frac{1}{\epsilon_\infty}\left(\epsilon_s + \frac{x^2}{(\omega_1h)^2}  \right)
	+ \frac{2}{\epsilon_\infty}\frac{x^2}{(\omega_1h)^2} 
	\right], \\
	q_1(x) &:= \frac{1}{\epsilon^2_\infty}\left(\epsilon_s + \frac{x^2}{(\omega_1h)^2}  \right)^2
	+ \frac{12}{\epsilon_\infty}
	\left( 1 - \WH{\gamma}^2 \right)\,\frac{x^2}{(\omega_1h)^2} ,  \\
	q_2(x) &:= -\frac{2}{\epsilon^3_\infty}\left(\epsilon_s + \frac{x^2}{(\omega_1h)^2}  \right)^3
	+ \frac{36}{\epsilon^2_\infty}\WH{\gamma}^2\left(\epsilon_s + \frac{x^2}{(\omega_1h)^2}  \right)\,\frac{x^2}{(\omega_1h)^2}  \notag \\
	& \hspace{.6cm}
	-\frac{108}{\epsilon_\infty}\frac{x^2}{(\omega_1h)^2} 
	\left[
	\WH{\gamma}^2 
	+ \frac{\WH{\gamma}^2}{\epsilon_\infty}\,\frac{x^2}{(\omega_1h)^2} 
	- \frac{2}{3\epsilon_\infty}\left(\epsilon_s + \frac{x^2}{(\omega_1h)^2}  \right)
	\right], 	  \\
	Q(x) &:= \left[
	\frac{1}{2}\left( q_2(x) + \sqrt{q_2^2(x)  - 4 q_1^3(x)} \right)
	\right]^{1/3},	 \\
	S(x) &:= \frac{1}{2}\left[
	-\frac{2}{3}P(x) + \frac{1}{3}\left( Q(x) + \frac{q_1(x)}{Q(x)} \right)
	\right]^{1/2}.		
	\end{align}
\end{subequations}

\noindent So the roots of equation \eqref{qq6} are given by
\begin{subequations}
	\label{Aex}
	\begin{align}
	\displaystyle
	\WH{\omega}^{\text{ex}}_{1}( \WH{k} )
	&= -\frac{i \WH{\gamma}}{2} - S(\WH{k}) 
	+ \frac{1}{2} \left[
	-4S^2(\WH{k}) - 2P(\WH{k}) + \frac{R(\WH{k})}{S(\WH{k})}
	\right]^{1/2},   \label{Aex1} \\
	\WH{\omega}^{\text{ex}}_{2}( \WH{k} )
	&= -\frac{i \WH{\gamma}}{2} - S(\WH{k}) 
	- \frac{1}{2} \left[
	-4S^2(\WH{k}) - 2P(\WH{k}) + \frac{R(\WH{k})}{S(\WH{k})}
	\right]^{1/2}, \label{Aex2} \\
	\WH{\omega}^{\text{ex}}_{3} (\WH{k})
	&= -\frac{i \WH{\gamma}}{2} + S(\WH{k}) 
	+ \frac{1}{2} \left[
	-4S^2(\WH{k}) - 2P(\WH{k}) - \frac{R(\WH{k})}{S(\WH{k})}
	\right]^{1/2}, \label{Aex3} \\
	\WH{\omega}^{\text{ex}}_{4} (\WH{k})
	&= -\frac{i \WH{\gamma}}{2} + S(\WH{k}) 
	- \frac{1}{2} \left[
	-4S^2(\WH{k}) - 2P(\WH{k}) - \frac{R(\WH{k})}{S(\WH{k})}
	\right]^{1/2}. \label{Aex4}
	\end{align}
\end{subequations}

\hspace{1cm}

\noindent Similarly, we consider the semi-discrete system \eqref{Dissemi3} based on the notations \eqref{Nota}:
\begin{align}
\displaystyle \label{qq7}
\sum_{p=1}^M \frac{[(2p-3)!!]^2}{(2p-1)!} 
\sin^{2p-1}\left( \frac{\WH{k}}{2} \right)
=
\frac{\omega_1h}{2}\,\WH{\omega}
\left[
\epsilon_\infty 
- \frac{\epsilon_d}{\WH{\omega}^2 + 2i\,\WH{\gamma}\,\WH{\omega} - 1}
\right]^{1/2}.
\end{align}

\noindent For convenience, we let 
$\displaystyle \textbf{F}(\WH{k}):= 
2\sum_{p=1}^M \frac{[(2p-3)!!]^2}{(2p-1)!} 
\sin^{2p-1}\left( \frac{\WH{k}}{2} \right)$. 
So from \eqref{qq7} and using the fact that  $\epsilon_d = \epsilon_s - \epsilon_\infty$, we obtain
\begin{align}
\displaystyle \label{qq8}
\textbf{F}^2 \left[
\WH{\omega}^2 + 2i\,\WH{\gamma}\,\WH{\omega} - 1
\right]
&=
\frac{(\omega_1 h)^2}{4}
\left[\epsilon_\infty \,\WH{\omega}^4 
+ 2\epsilon_\infty\, i \,\WH{\gamma}\, \WH{\omega}^3
- \epsilon_s\, \WH{\omega}^2 \right].
\end{align}

\noindent Simplifying equation \eqref{qq8}, we get
\begin{align}
\displaystyle \label{qq9}
\WH{\omega}^4 
+ 2i\,\WH{\gamma}\,\WH{\omega}^3 
- \frac{1}{\epsilon_\infty}
\left(
\epsilon_s + \frac{\textbf{F}^2}{(\omega_1 h)^2}
\right) \WH{\omega}^2
- \frac{2i}{\epsilon_\infty} \WH{\gamma}\, \frac{\textbf{F}^2}{(\omega_1 h)^2}\, \WH{\omega}
+ \frac{1}{\epsilon_\infty} \frac{\textbf{F}^2}{(\omega_1 h)^2}= 0.
\end{align}

\noindent Similarly process to find the roots of the exact dispersion relation, all roots of equation \eqref{qq9} are
\begin{subequations}
	\label{AFD}
	\begin{align}
	\displaystyle
	\WH{\omega}^{\text{FD}}_{1}( \WH{k} )
	&= -\frac{i \WH{\gamma}}{2} - S(\textbf{F}( \WH{k} )) 
	+ \frac{1}{2} \left[
	-4S^2(\textbf{F}( \WH{k} )) - 2P(\textbf{F}( \WH{k} )) + \frac{R(\textbf{F}( \WH{k} ))}{S(\textbf{F}( \WH{k} ))}
	\right]^{1/2},  	\label{AFD1}\\
	\WH{\omega}^{\text{FD}}_{2}( \WH{k} )
	&= -\frac{i \WH{\gamma}}{2} - S(\textbf{F}( \WH{k} )) 
	- \frac{1}{2} \left[
	-4S^2(\textbf{F}( \WH{k} )) - 2P(\textbf{F}( \WH{k} )) + \frac{R(\textbf{F}( \WH{k} ))}{S(\textbf{F}( \WH{k} ))}
	\right]^{1/2},  	\label{AFD2}\\
	\WH{\omega}^{\text{FD}}_{3} (\WH{k})
	&= -\frac{i \WH{\gamma}}{2} + S(\textbf{F}( \WH{k} )) 
	+ \frac{1}{2} \left[
	-4S^2(\textbf{F}( \WH{k} )) - 2P(\textbf{F}( \WH{k} )) - \frac{R(\textbf{F}( \WH{k} ))}{S(\textbf{F}( \WH{k} ))}
	\right]^{1/2}, 	\label{AFD3}\\
	\WH{\omega}^{\text{FD}}_{4} (\WH{k})
	&= -\frac{i \WH{\gamma}}{2} + S(\textbf{F}( \WH{k} )) 
	- \frac{1}{2} \left[
	-4S^2(\textbf{F}( \WH{k} )) - 2P(\textbf{F}( \WH{k} )) - \frac{R(\textbf{F}( \WH{k} ))}{S(\textbf{F}( \WH{k} ))}
	\right]^{1/2}. 	\label{AFD4}
	\end{align}
\end{subequations}

We plot the relative phase error and the ratio of $|\omega^{FD}/\omega^{ex}|$ of all roots for both exact and FD dispersion system with all following parameters
\begin{itemize}
	\item $\epsilon_s = 5.25$
	\item $\epsilon_\infty = 2.25$
	\item $\omega_1 h = \frac{\pi}{30}$
	\item Domain $\Omega = [0,2\pi]$
\end{itemize}

\newpage

\noindent We present the numerical experiment of the dispersion relations depending on the parameter $\gamma$.\\

\noindent \textbf{Case 1:} $\displaystyle \WH{\gamma} = \frac{\gamma}{\omega_1} = 0$

In this case, we see that equation \eqref{Aex} has the following relationships
\begin{subequations}
	\label{B1}
	\begin{align}
	\WH{\omega}^{\text{ex}}_{1}( \WH{k} ) + \WH{\omega}^{\text{ex}}_{4}( \WH{k} )&= 0, \\
		\WH{\omega}^{\text{ex}}_{2}( \WH{k} ) + \WH{\omega}^{\text{ex}}_{3}( \WH{k} )&= 0. 
	\end{align}
\end{subequations}

\noindent Moreover, equation \eqref{AFD} has the following relationships
\begin{subequations}
		\label{B2}
	\begin{align}
	\WH{\omega}^{\text{FD}}_{1}( \WH{k} ) + \WH{\omega}^{\text{FD}}_{4}( \WH{k} )&= 0, \\
	\WH{\omega}^{\text{FD}}_{2}( \WH{k} ) + \WH{\omega}^{\text{FD}}_{3}( \WH{k} )&= 0. 
	\end{align}
\end{subequations} 

\noindent We demonstrate the behavior of each equation \eqref{B1} and \eqref{B2} in Figure \ref{Fig: A1} and Figure \ref{Fig: A2}. It also answers why the relative phase error for the case $i=1$ and $i=4$ (also the case $i=2$ and $i=3$) in Figure \ref{Fig: A2} are identical.
 
\begin{figure}[H]
	\centering
	\includegraphics[scale=0.55]{pics/EX_g0}
	\includegraphics[scale=0.55]{pics/FD_g0} 
	\caption{Real part and imaginary part of $\WH{\omega}^{\text{ex}}_{i}( \WH{k} )$ and $\WH{\omega}^{\text{FD}}_{i}( \WH{k} )$ for FD2 where $i = 1,2,3,4$ }
	\label{Fig: A1}
\end{figure}

\begin{figure}[H]
	\centering
	\includegraphics[scale=0.27]{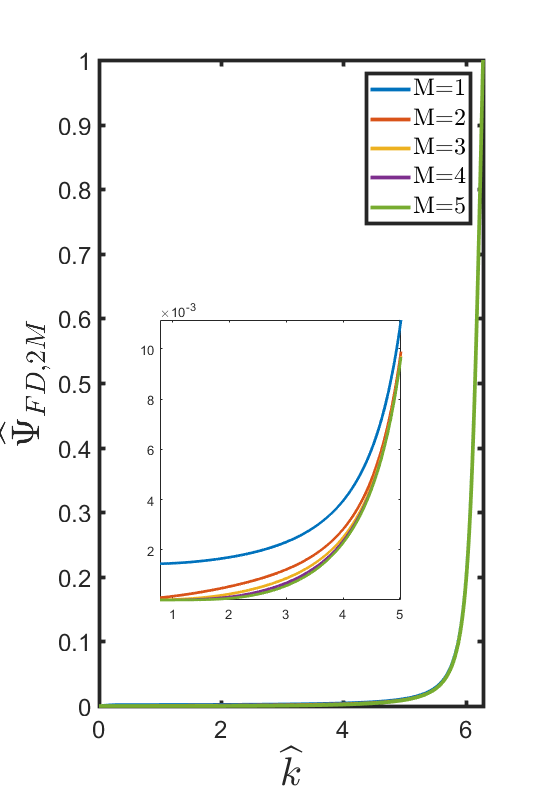}
	\includegraphics[scale=0.27]{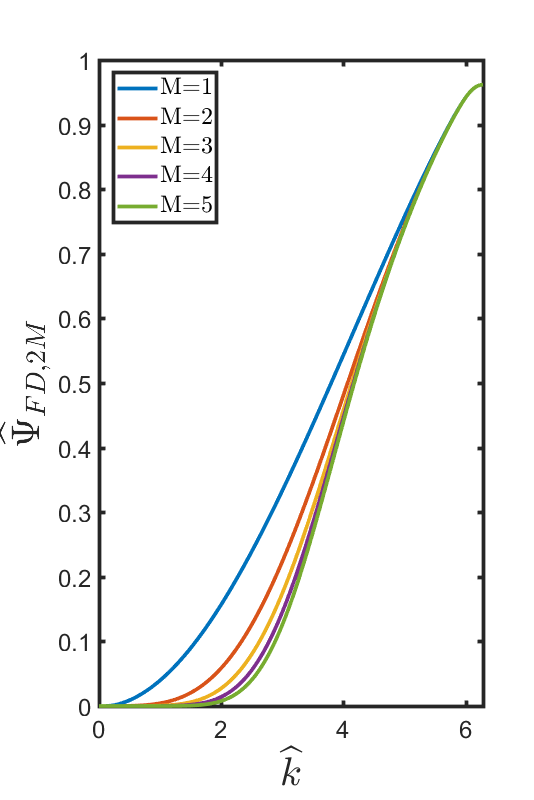} 
	\includegraphics[scale=0.27]{pics/RelE3_g0}
	\includegraphics[scale=0.27]{pics/RelE4_g0}
	\caption{Relative Error: $\displaystyle 
		\left| \frac{ \WH{\omega}^{\text{ex}}_{i} - \WH{\omega}^{\text{FD}}_{i}}{ \WH{\omega}^{\text{ex}}_{i}} \right|$ for $ i = 1,2,3,4$}
		\label{Fig: A2}
\end{figure}

%\begin{figure}[H]
%	\centering
%	\includegraphics[scale=0.27]{pics/RatE1_g0}
%	\includegraphics[scale=0.27]{pics/RatE2_g0} 
%	\includegraphics[scale=0.27]{pics/RatE3_g0}
%	\includegraphics[scale=0.27]{pics/RatE4_g0}
%	\caption{Relative Error: $\displaystyle \left| \frac{ \WH{\omega}^{\text{FD}}_{i}}{ \WH{\omega}^{\text{ex}}_{i}} \right|$ for $ i = 1,2,3,4$}
%\end{figure}

\newpage
\noindent \textbf{Case 2:} $\WH{\gamma} = \frac{\gamma}{\omega_1} = 0.01$

In this case, we will analyze the system \eqref{B1} and \eqref{B2} as in the case $\WH{\gamma} = 0$. In Figure \ref{Fig: B1}, we obtain the following relations for the case $i=1$ and $i=4$ (also the case $i=2$ and $i=3$), i.e. the real part of the first (second) root and the fourth (third) root are negative to each other:
\begin{subequations}
	\label{C}
	\begin{align}
	\Re \left( \WH{\omega}^{\text{ex}}_{1}( \WH{k} ) + \WH{\omega}^{\text{ex}}_{4}( \WH{k} ) \right) &= 0, \quad
	\Re \left( \WH{\omega}^{\text{ex}}_{2}( \WH{k} ) + \WH{\omega}^{\text{ex}}_{3}( \WH{k} ) \right) = 0, \\
	\Re \left( \WH{\omega}^{\text{FD}}_{1}( \WH{k} ) + \WH{\omega}^{\text{FD}}_{4}( \WH{k} ) \right) &= 0, \quad
	\Re \left( \WH{\omega}^{\text{FD}}_{2}( \WH{k} ) + \WH{\omega}^{\text{FD}}_{3}( \WH{k} ) \right) = 0. 
	\end{align}
\end{subequations}

\noindent Moreover, for the imaginary part, we have the following relationships
\begin{subequations}
	\label{D}
	\begin{align}
	\Im \left( \WH{\omega}^{\text{ex}}_{1}( \WH{k} ) - \WH{\omega}^{\text{ex}}_{4}( \WH{k} ) \right) &= 0, \quad
	\Im \left( \WH{\omega}^{\text{ex}}_{2}( \WH{k} ) - \WH{\omega}^{\text{ex}}_{3}( \WH{k} ) \right) = 0, \\
	\Im \left( \WH{\omega}^{\text{FD}}_{1}( \WH{k} ) - \WH{\omega}^{\text{FD}}_{4}( \WH{k} ) \right) &= 0, \quad
	\Im \left( \WH{\omega}^{\text{FD}}_{2}( \WH{k} ) - \WH{\omega}^{\text{FD}}_{3}( \WH{k} ) \right) = 0,
	\end{align}
\end{subequations}

\noindent which is shown in Figure \ref{Fig: B2}. Base on the fact of relationships \eqref{C} and \eqref{D}, if we assume $\WH{\omega}_i$ be the $i$-th root of system \eqref{Aex} or \eqref{AFD} for $i=1,2,3,4$, then 
\begin{subequations}
	\label{E}
	\begin{align}
	\displaystyle
	\WH{\omega}_1
	&= a + bi,
	&& \WH{\omega}_4
	= -a + bi 
	= - \overline{\WH{\omega}_1}, \\
	\WH{\omega}_2
	&= c + di,
	&& \WH{\omega}_3
	= -c + di
	= - \overline{\WH{\omega}_2},
	\end{align}
\end{subequations}

\noindent for some real values $a,b,c$ and $d$. In fact, the identity \eqref{E} also satisfies the conjugate root theorem of the system \eqref{Aex} and \eqref{AFD} for the loss less material $\WH{\gamma} <<1$. 
However, for the higher value of $\WH{\gamma} >>1$, the types of roots in \eqref{Aex} or \eqref{AFD} depend on $\WH{k}$:
\begin{itemize}
	\item \textbf{Case 1:} $\WH{k}$ is small enough, $\WH{k} << c$ where $c$ is a real number. The roots in \eqref{Aex} or \eqref{AFD} also satisfy the relationship \eqref{E}.
	\item \textbf{Case 1:} $\WH{k}$ is big enough, $\WH{k} >> c$. The roots in \eqref{Aex} or \eqref{AFD} consist of 4 complex numbers; two roots have different purely imaginary parts and the other are $z$ and its $-\overline{z}$.
\end{itemize}

\noindent From the identity \eqref{E}, we can show that 
\begin{subequations}
	\label{F}
	\begin{align}
	\displaystyle
	\left| \frac{\WH{\omega}^{ex}_1 - \WH{\omega}^{FD}_1}{\WH{\omega}^{ex}_1} \right|
	&= 	\left| \frac{\WH{\omega}^{ex}_4 - \WH{\omega}^{FD}_4}{\WH{\omega}^{ex}_4} \right|, \\
	\left| \frac{\WH{\omega}^{ex}_2 - \WH{\omega}^{FD}_2}{\WH{\omega}^{ex}_2} \right|
	&= 	\left| \frac{\WH{\omega}^{ex}_3 - \WH{\omega}^{FD}_3}{\WH{\omega}^{ex}_3} \right|.	
	\end{align}
\end{subequations}

\noindent Furthermore, for the higher value of $\WH{\gamma} >>1$, the relationship \eqref{F} does not hold because of two roots having different purely imaginary parts. For the behavior of the other, the relative phase error will be identical in some domain of $\WH{k}$.

In this case with the relationship \eqref{E}, it implies that the relative phase error of the first (second) and the forth (third) root are identical, which is shown in Figure \ref{Fig: B3}

\begin{figure}[H]
	\centering
	\includegraphics[scale=0.55]{pics/EX_g01}
	\includegraphics[scale=0.55]{pics/FD_g01} 
	\caption{Real part and imaginary part of $\WH{\omega}^{\text{ex}}_{i}( \WH{k} )$ and $\WH{\omega}^{\text{FD}}_{i}( \WH{k} )$ for FD2 where $i = 1,2,3,4$ }
	\label{Fig: B1}
\end{figure}

\begin{figure}[H]
	\centering
	\includegraphics[scale=0.55]{pics/EX_g01_2}
	\includegraphics[scale=0.55]{pics/FD_g01_2} 
	\caption{Real part and imaginary part of $\WH{\omega}^{\text{ex}}_{i}( \WH{k} )$ and $\WH{\omega}^{\text{FD}}_{i}( \WH{k} )$ for FD2 where $i = 1,2,3,4$ }
	\label{Fig: B2}
\end{figure}

\begin{figure}[H]
	\centering
	\includegraphics[scale=0.27]{pics/RelE1_g01}
	\includegraphics[scale=0.27]{pics/RelE2_g01} 
	\includegraphics[scale=0.27]{pics/RelE3_g01}
	\includegraphics[scale=0.27]{pics/RelE4_g01}
	\caption{Relative Error: $\displaystyle 
		\left| \frac{ \WH{\omega}^{\text{ex}}_{i} - \WH{\omega}^{\text{FD}}_{i}}{ \WH{\omega}^{\text{ex}}_{i}} \right|$ for $ i = 1,2,3,4$}
	\label{Fig: B3}
\end{figure}

From the above analysis, we see that the numerical dispersion error in low loss material is not much different lossless materials. However, the relative phase error of the first (second) and the fourth (third) root are identical for low loss material $\WH{\gamma}$. To compare among the order of scheme, the phase error of the scheme has no significant difference for $M \geq 3$. Hence the analysis of $\omega(k)$ also supports that the forth order scheme is the "best" scheme to work with like in Section 5.

%\begin{figure}[H]
%	\centering
%	\includegraphics[scale=0.27]{pics/RatE1}
%	\includegraphics[scale=0.27]{pics/RatE2} 
%	\includegraphics[scale=0.27]{pics/RatE3}
%	\includegraphics[scale=0.27]{pics/RatE4}
%	\caption{Relative Error: $\displaystyle \left| \frac{ \WH{\omega}^{\text{FD}}_{i}}{ \WH{\omega}^{\text{ex}}_{i}} \right|$ for $ i = 1,2,3,4$}
%\end{figure}
