# Supplementary material for: Dispersion Analysis of Finite Difference and Discontinuous Galerkin Schemes for Maxwell's Equations in Linear Lorentz Media
Source: arXiv:1810.01723 source file (2018-10-03)
Supplement: Supplementary file 2 [file appendix2.tex]

\section{ Four physical quantities with other fully discrete schemes} \label{sec:phy_add}
\YJ{ change title}

\begin{figure}[H]
	\centering
	\includegraphics[scale=0.25]{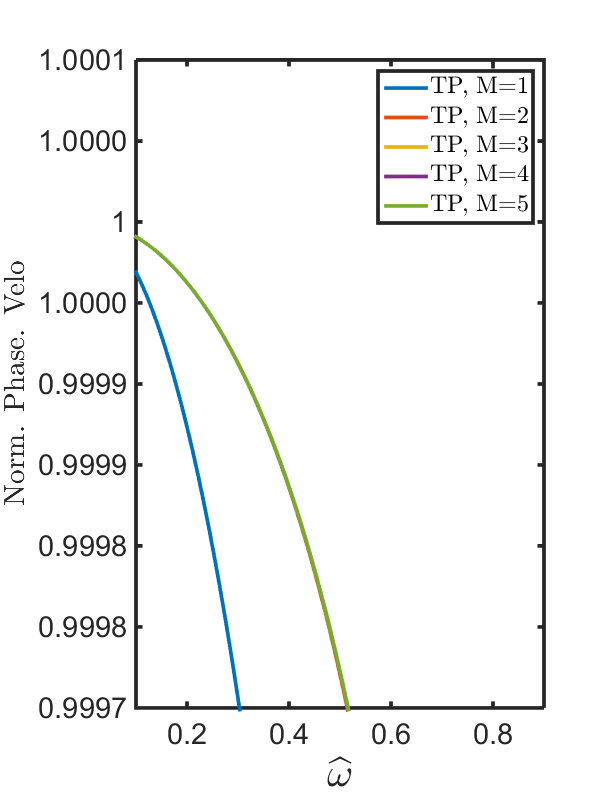}
	\includegraphics[scale=0.25]{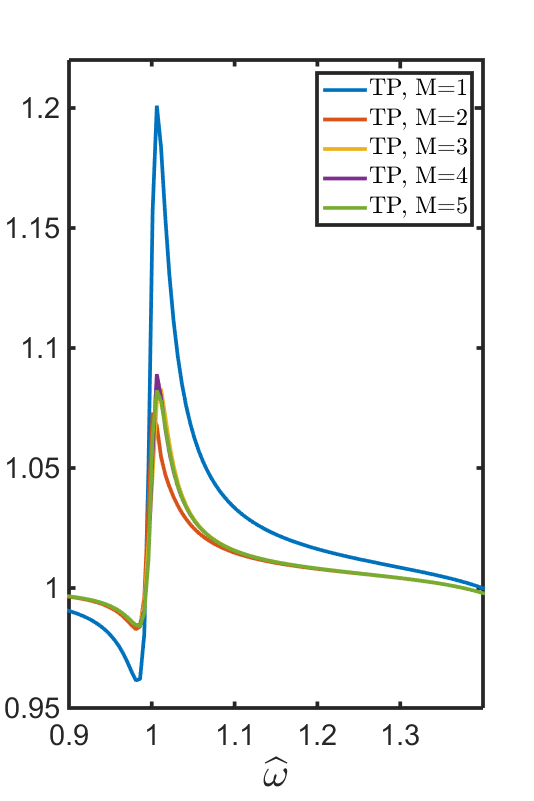}
	\includegraphics[scale=0.25]{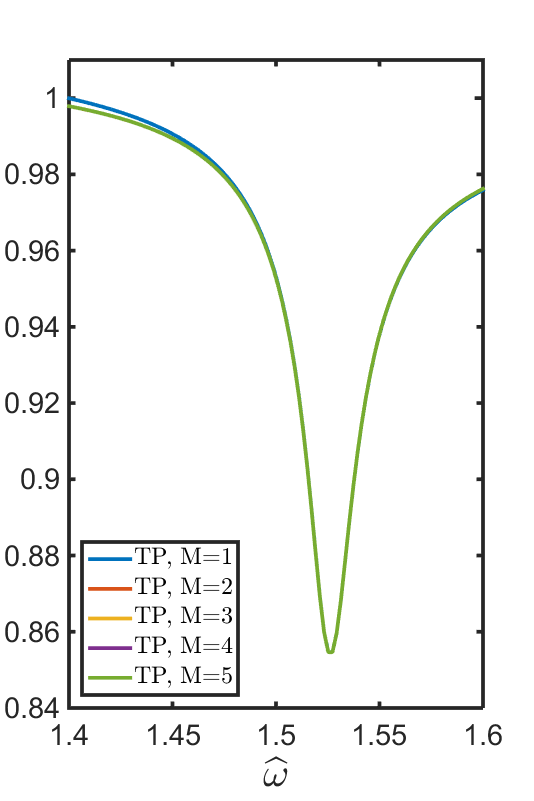}
	\includegraphics[scale=0.25]{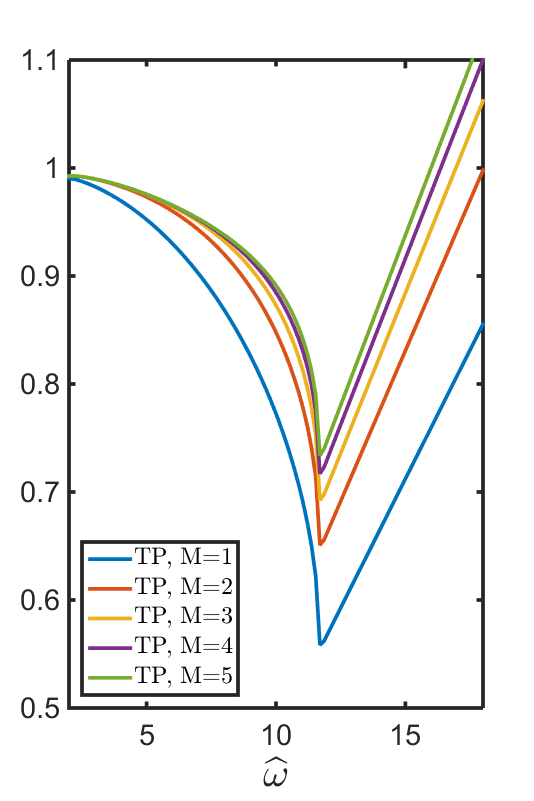} \\
	\includegraphics[scale=0.25]{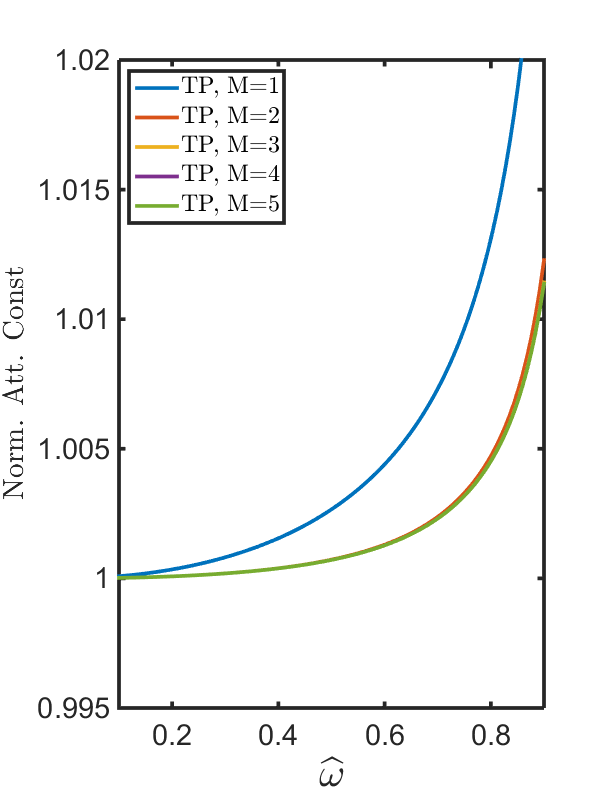}
	\includegraphics[scale=0.25]{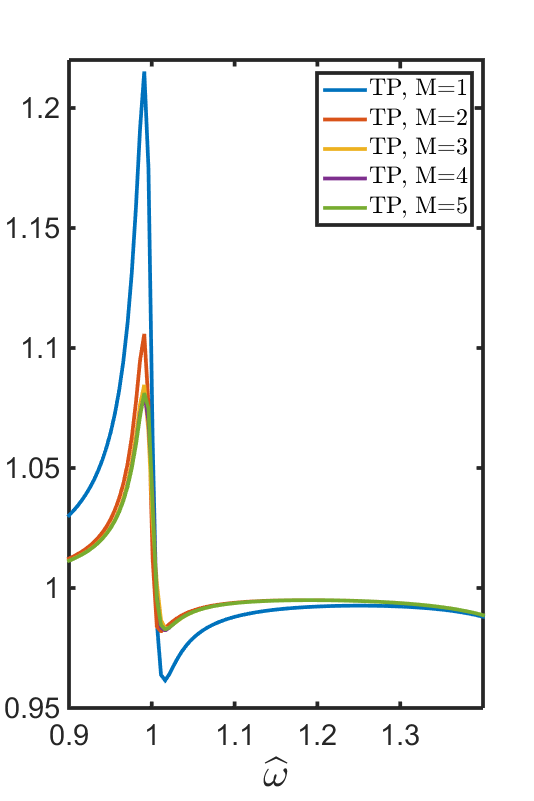}
	\includegraphics[scale=0.25]{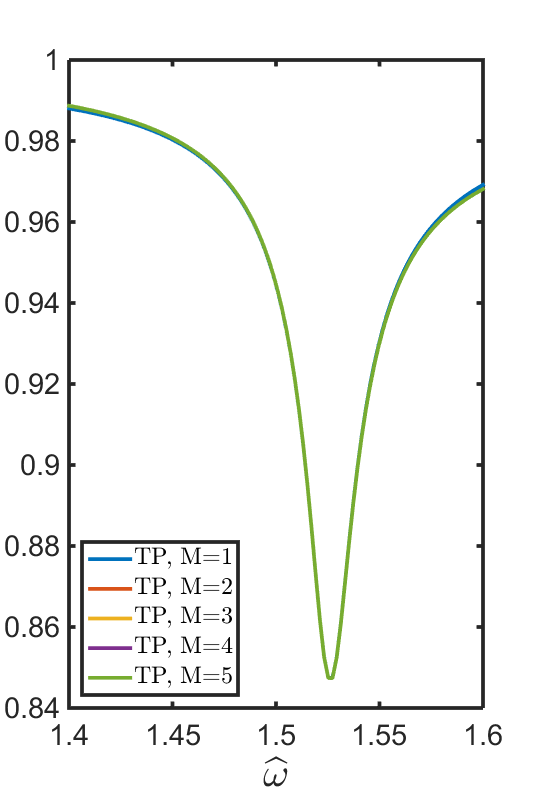}
	\includegraphics[scale=0.25]{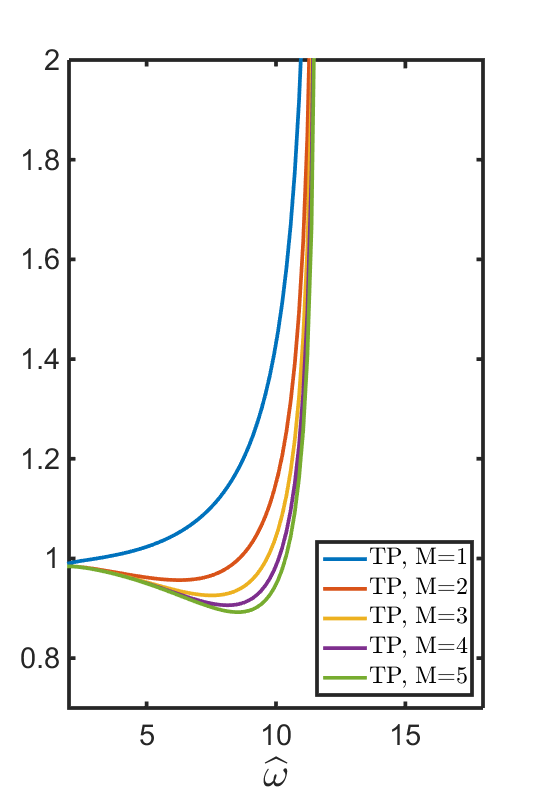} \\
	%	%
	\includegraphics[scale=0.25]{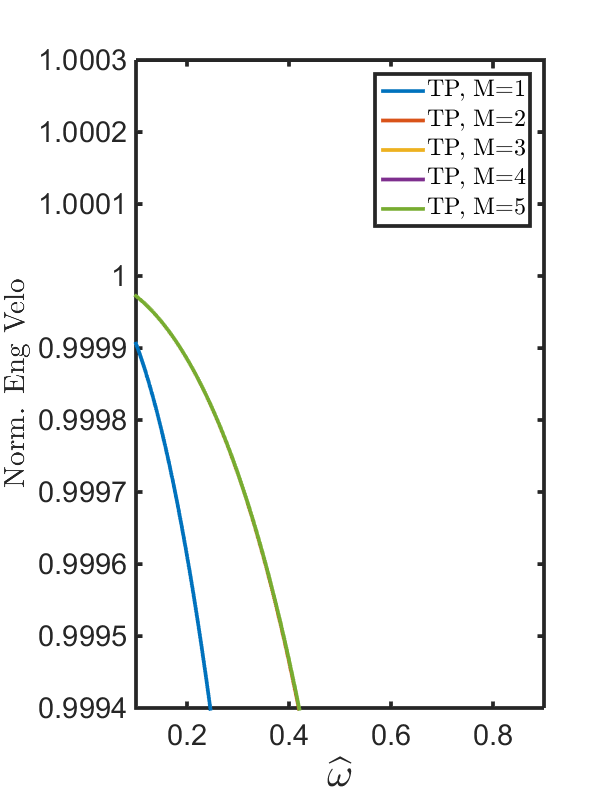}
	\includegraphics[scale=0.25]{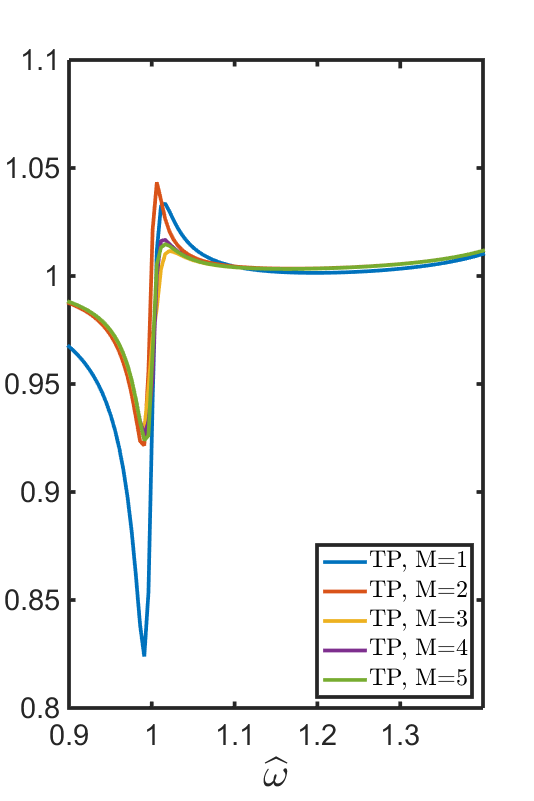}
	\includegraphics[scale=0.25]{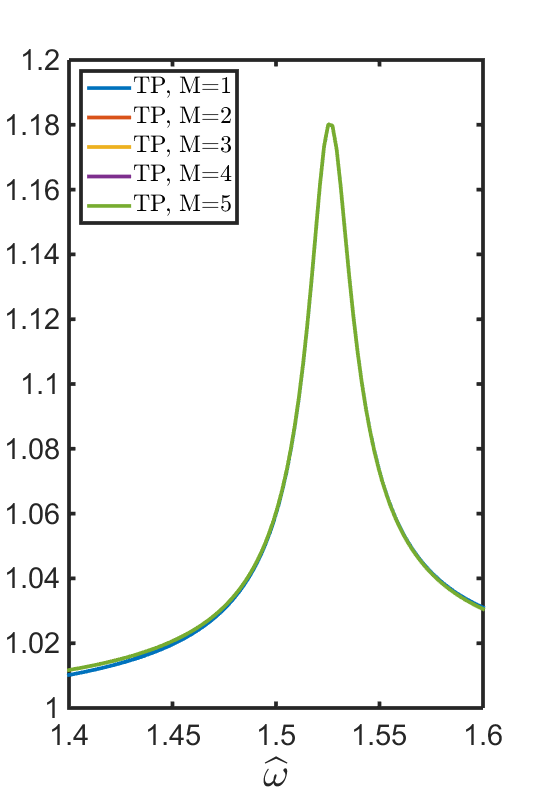}
	\includegraphics[scale=0.25]{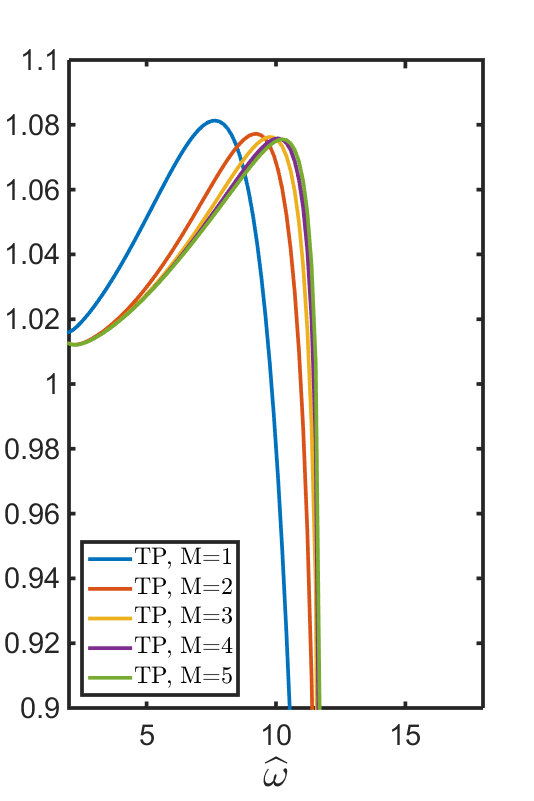} \\
	%	%
	\includegraphics[scale=0.25]{pics/GpVelo_FullTP1_v2}
	\includegraphics[scale=0.25]{pics/GpVelo_FullTP2_v2}
	\includegraphics[scale=0.25]{pics/GpVelo_FullTP3_v2}
	\includegraphics[scale=0.25]{pics/GpVelo_FullTP4_v2} \\	
	\caption{Dispersion relations for trapezoidal scheme of FD with CFL number $\nu/\nu^{M}_{\max}=0.7$. First row: Normalized phase velocity, second row: normalized attenuation constants, third row: normalized energy velocity, forth row: normalized group velocity  }
	\label{Fig:FD_TP_phy}
\end{figure}

\begin{figure}[H]
	\centering
	\includegraphics[scale= 0.25] {pics/Phase_Velo_TP_AL_1.eps}
	\includegraphics[scale= 0.25] {pics/Phase_Velo_TP_AL_2.eps}
	\includegraphics[scale= 0.25] {pics/Phase_Velo_TP_AL_3.eps}
	\includegraphics[scale= 0.25] {pics/Phase_Velo_TP_AL_4.eps}	
	\includegraphics[scale= 0.25] {pics/Att_Const_TP_AL_1.eps}
	\includegraphics[scale= 0.25] {pics/Att_Const_TP_AL_2.eps}
	\includegraphics[scale= 0.25] {pics/Att_Const_TP_AL_3.eps}
	\includegraphics[scale= 0.25] {pics/Att_Const_TP_AL_4.eps}
	\includegraphics[scale= 0.25] {pics/Eng_Velo_TP_AL_1.eps}
	\includegraphics[scale= 0.25] {pics/Eng_Velo_TP_AL_2.eps}
	\includegraphics[scale= 0.25] {pics/Eng_Velo_TP_AL_3.eps}
	\includegraphics[scale= 0.25] {pics/Eng_Velo_TP_AL_4.eps}
	\includegraphics[scale= 0.25] {pics/Group_Velo_TP_AL_1.eps}
	\includegraphics[scale= 0.25] {pics/Group_Velo_TP_AL_2.eps}
	\includegraphics[scale= 0.25] {pics/Group_Velo_TP_AL_3.eps}
	\includegraphics[scale= 0.25] {pics/Group_Velo_TP_AL_4.eps}
	\caption{The physical quantities for trapezoidal scheme of with CFL number DG-AL$\nu/\nu^{M}_{\max}=0.7$. First row: Normalized phase velocity, second row: normalized attenuation constants, third row: normalized energy velocity, forth row: normalized group velocity  }
	\label{Fig:AL_TP_phy}
\end{figure}

%\begin{figure}[H]
%	\centering
%	\includegraphics[scale= 0.25] {pics/Phase_Velo_LP_CE_1.eps}
%	\includegraphics[scale= 0.25] {pics/Phase_Velo_LP_CE_2.eps}
%	\includegraphics[scale= 0.25] {pics/Phase_Velo_LP_CE_3.eps}
%	\includegraphics[scale= 0.25] {pics/Phase_Velo_LP_CE_4.eps}
%	\includegraphics[scale= 0.25] {pics/Att_Const_LP_CE_1.eps}
%	\includegraphics[scale= 0.25] {pics/Att_Const_LP_CE_2.eps}
%	\includegraphics[scale= 0.25] {pics/Att_Const_LP_CE_3.eps}
%	\includegraphics[scale= 0.25] {pics/Att_Const_LP_CE_4.eps}
%	\includegraphics[scale= 0.25] {pics/Eng_Velo_LP_CE_1.eps}
%	\includegraphics[scale= 0.25] {pics/Eng_Velo_LP_CE_2.eps}
%	\includegraphics[scale= 0.25] {pics/Eng_Velo_LP_CE_3.eps}
%	\includegraphics[scale= 0.25] {pics/Eng_Velo_LP_CE_4.eps}
%	\includegraphics[scale= 0.25] {pics/Group_Velo_LP_CE_1.eps}
%	\includegraphics[scale= 0.25] {pics/Group_Velo_LP_CE_2.eps}
%	\includegraphics[scale= 0.25] {pics/Group_Velo_LP_CE_3.eps}
%	\includegraphics[scale= 0.25] {pics/Group_Velo_LP_CE_4.eps}
%	\caption{The physical quantities for leap-frog of DG-CE with CFL number $\nu/\nu^{M}_{\max}=0.7$ First row: Normalized phase velocity, second row: normalized attenuation constants, third row: normalized energy velocity, forth row: normalized group velocity  }
%	\label{Fig:CE_LF_phy}
%\end{figure}

\begin{figure}[H]
	\centering
	\includegraphics[scale= 0.25] {pics/Phase_Velo_TP_CE_1.eps}
	\includegraphics[scale= 0.25] {pics/Phase_Velo_TP_CE_2.eps}
	\includegraphics[scale= 0.25] {pics/Phase_Velo_TP_CE_3.eps}
	\includegraphics[scale= 0.25] {pics/Phase_Velo_TP_CE_4.eps}
	\includegraphics[scale= 0.25] {pics/Att_Const_TP_CE_1.eps}
	\includegraphics[scale= 0.25] {pics/Att_Const_TP_CE_2.eps}
	\includegraphics[scale= 0.25] {pics/Att_Const_TP_CE_3.eps}
	\includegraphics[scale= 0.25] {pics/Att_Const_TP_CE_4.eps}
	\includegraphics[scale= 0.25] {pics/Eng_Velo_TP_CE_1.eps}
	\includegraphics[scale= 0.25] {pics/Eng_Velo_TP_CE_2.eps}
	\includegraphics[scale= 0.25] {pics/Eng_Velo_TP_CE_3.eps}
	\includegraphics[scale= 0.25] {pics/Eng_Velo_TP_CE_4.eps}
	\includegraphics[scale= 0.25] {pics/Group_Velo_TP_CE_1.eps}
	\includegraphics[scale= 0.25] {pics/Group_Velo_TP_CE_2.eps}
	\includegraphics[scale= 0.25] {pics/Group_Velo_TP_CE_3.eps}
	\includegraphics[scale= 0.25] {pics/Group_Velo_TP_CE_4.eps}
	\caption{The physical quantities for trapezoidal scheme of DG-CE with CFL number $\nu/\nu^{M}_{\max}=0.7$ First row: Normalized phase velocity, second row: normalized attenuation constants, third row: normalized energy velocity, forth row: normalized group velocity  }
	\label{Fig:CE_TP_phy}
\end{figure}
