# Supplementary material for: Dispersion Analysis of Finite Difference and Discontinuous Galerkin Schemes for Maxwell's Equations in Linear Lorentz Media
Source: arXiv:1810.01723 source file (2018-10-03)
Supplement: Supplementary file 3 [file appendix_2.tex]

%\newpage
%\section{Analyze Physical and Spurious Modes of Fully Discrete Scheme}
%
%
%Recall notations:
%\begin{itemize}
%	\item $W = \omega \Delta t;\quad \hat{\omega} = \frac{\omega}{\omega_1};
%	\quad \hat{\gamma} = \frac{\gamma}{\omega_1}; \quad K = k^{ex}h $
%	\item $\displaystyle \delta(\hat{\omega};\textbf{p}) 
%	= \frac{\epsilon_d \hat{\omega} (\hat{\omega} + i\hat{\gamma})}{(-1 + 2i\hat{\gamma}\hat{\omega} + \hat{\omega}^2)^2}$ 
%	
%	\textcolor{red}{\textbf{Condition: New definition !!}}
%	\item Eq (4.4): 
%	\[\displaystyle
%	k^{LF} = \pm k^{ex}\left(
%	1 + \frac{1}{12}\left( \frac{\delta}{\epsilon} - \frac{1}{2} \right)W^2
%	+ \mathcal{O}(W^4)
%	\right)
%	\]
%	\textcolor{red}{\textbf{Condition: Assume the previous definition holds !!}}
%%	\item Eq (5.22) only for LF method
%%	\begin{align}
%%	\displaystyle
%%	\sum_{p=1}^M 
%%	\frac{[(2p-3)!!]^2}{(2p-1)!} \sin^{2p-1}\left( \frac{k_{FD}^{LF}h}{2} \right)
%%	&= \frac{k^{LF}h}{2} \notag \\
%%	&=\frac{K}{2}\left(
%%	1 + \frac{1}{12}\left( \frac{\delta}{\epsilon} - \frac{1}{2} \right)W^2
%%	+ \mathcal{O}(W^4)
%%	\right) \label{qqq1}
%%	\end{align}
%%	%
%%	\item Eq (5.26) only for TP method
%%	\begin{align}
%%	\displaystyle
%%	\sum_{p=1}^M 
%%	\frac{[(2p-3)!!]^2}{(2p-1)!} \sin^{2p-1}\left( \frac{k_{FD}^{TP}h}{2} \right)
%%	&= \frac{k^{TP}h}{2} \notag \\
%%	&=\frac{K}{2}\left(
%%	1 + \frac{1}{12}\left( \frac{\delta}{\epsilon} + 1\right)W^2
%%	+ \mathcal{O}(W^4)
%%	\right) \label{qqq2}
%%	\end{align}
%\end{itemize}
%
%
%
%%
%%\noindent \textbf{Analyze the Spurious modes for Fully discrete scheme M = 1:}
%%
%%For $M = 1$, we get 
%%\[\displaystyle
%%\sin\left( \frac{k^{\text{LF}}_{\text{FD}}h}{2} \right)
%%= \frac{K}{2}\left(
%%1 + \frac{1}{12}\left( \frac{\delta(\hat{\omega};\textbf{p})}{\epsilon(\hat{\omega};\textbf{p})} - \frac{1}{2} \right)W^2
%%+ \mathcal{O}(W^4)
%%\right)
%%\]
%
%
%\noindent From equation \eqref{eq:dis_LF} and \eqref{eq:dis_TP}, we first let some notations
%%\noindent From equation \eqref{DisLF7} and \eqref{DisTP7}, we first let some notations
%\begin{align*}
%\displaystyle
%r_{_{LF}}(W) &= 
%1+ \frac{1}{12}\left( \frac{\delta(\hat{\omega};\textbf{p})}{\epsilon(\hat{\omega};\textbf{p})} - \frac{1}{2} \right)W^2
%\Leftrightarrow  
%k^{\text{LF}} = k^{\text{ex}}r_{_{LF}}(W), \\
%%
%r_{_{TP}}(W) &= 
%1+ \frac{1}{12}\left( \frac{\delta(\hat{\omega};\textbf{p})}{\epsilon(\hat{\omega};\textbf{p})} + 1 \right)W^2
%\Leftrightarrow  
%k^{\text{TP}} = k^{\text{ex}}r_{_{TP}}(W).
%\end{align*}
%
%
%
%\noindent From equation \eqref{DisLF7}, then the Taylor expansion of
%the physical, $k^{\text{LF}}_{\text{FD}}$ of the fully discrete dispersion where $K \approx 0$ are given by
%\begin{itemize}
%	\item For physical modes for $M \geq 1$
%	\begin{align}
%	\displaystyle 
%	k^{\text{LF}}_{\text{FD},p}
%	&=  k^{ex}\Big[
%	r_{_{LF}}(W) + \frac{[(2M-1)!!]^2}{2^{2M}(2M+1)!}K^{2M}r_{_{LF}}^{2M+1}(W) 
%	+  \mathcal{O}(K^{2M+2}r_{_{LF}}^{2M+3}(W) )  
%	\Big], 	\label{phy1:LF} 
%	\end{align}	
%
%
%	\item For spurious modes where $M = 2$
%	\begin{subequations}
%		\label{slf2}	
%	\begin{align}
%	\displaystyle
%	k^{\text{LF}}_{\text{FD},s_1}
%	&= k^{ex}
%	\Big[
%	\frac{2i}{K}\text{arcsinh}(\sqrt{6})
%	-\frac{r_{_{LF}}(W)}{2\sqrt{7}} 
%	+ \sqrt{\frac{3}{14}}\cdot \frac{9i}{112}Kr_{_{LF}}^2(W) 
%	+ \frac{45K^2}{1568\sqrt{7}}r_{_{LF}}^3(W)     \notag \\
%	& \hspace{ 1.2 cm } - \frac{5685}{702464}\sqrt{\frac{3}{14}}iK^3r_{_{LF}}^4(W)  
%	+  \mathcal{O}(K^4r_{_{LF}}^5(W))  
%	\Big],    \label{slf1} \\
%	%
%	k^{\text{LF}}_{\text{FD},s_2}
%	&= \overline{	k^{\text{LF}}_{\text{FD},s_1}}.  
%	\end{align}
%		\end{subequations}
%	\textbf{Note:} To find the general (explicit) form of spurious modes for $M >2$ is quite difficult.
%\end{itemize}
%
%
%
%
%\noindent Using the relationship $\displaystyle K = \frac{1}{v}\sqrt{\frac
%	{\epsilon(\hat{\omega};\textbf{p})}{\epsilon_\infty}}W$, we can treated physical solutions \eqref{phy1:LF} and spurious solutions \eqref{slf2}  as a function of $W$ as
%\begin{itemize}
%	\item For physical modes
%	\begin{align}
%	\displaystyle k^{\text{LF}}_{\text{FD},p}
%	= 
%	\begin{cases}
%	\displaystyle k^{ex}
%	\left(
%	1 + 
%	\frac{1}{12}\left( \frac{\delta(\hat{\omega};\textbf{p})}{\epsilon(\hat{\omega};\textbf{p})} - \frac{1}{2} + \frac{\epsilon(\hat{\omega}:\textbf{p})}{2\epsilon_\infty\nu^2}\right)W^2
%	+ \mathcal{O}(W^4)
%	\right)  &; M = 1, \\ \\
%	% 
%	\displaystyle
%	k^{ex}
%	\Big(
%	r_{_{LF}}(W)
%	+ \frac{[(2M-1)!!]^2}{2^{2M}(2M+1)!}\left( \frac{\epsilon(\WH{\omega};\textbf{p})}{\epsilon_\infty \nu^2} \right)^M W^{2M}
%	+  \mathcal{O}(W^{2M+2})  
%	\Big)  &; M \geq 2. 
%	\end{cases}    \label{pplf1}
%	\end{align}
%	\item For spurious modes $M = 2$
%	\begin{align}
%	\displaystyle
%	k^{\text{LF}}_{\text{FD},s_1}
%	&= k^{ex}
%	\Big[
%	\sqrt{\frac{\epsilon_\infty}{\epsilon(\hat{\omega};\textbf{p})}}\frac{2\nu i}{W}\text{arcsinh}(\sqrt{6})
%	+ 
%	\left( -\frac{1}{2\sqrt{7}} + \frac{9i}{112\nu}\sqrt{\frac{3\epsilon(\hat{\omega};\textbf{p})}{14\epsilon_\infty}} \right)W
%	+  \mathcal{O}(W^2)  
%	\Big],  \label{sslf1}\\
%	%
%	k^{\text{LF}}_{\text{FD},s_2} 
%	&= \overline{	k^{\text{LF}}_{\text{FD},s_1}}. \label{sslf2}
%	\end{align}
%\end{itemize} 
%
%
%
%By observing that we found that the discrete dispersion relation is in the form of odd power degree polynomial. As $K \approx 0$, the roots of such polynomial consist of only one real root and pairs of complex numbers. The real roots presents a physical mode while the pairs of complex numbers provide spurious modes. That's why it's enough to focus the behavior of higher order scheme by using the case $M=2$.
% 
% 
%Similarly the physical and spurious modes for trapezoidal scheme \eqref{DisTP7} where $K \approx 0$ are written in the form 
%\begin{itemize}
%	\item For physical modes for $M \geq 1$
%	\begin{align}
%	\displaystyle 
%	k^{\text{TP}}_{\text{FD},p}
%	&=  k^{ex}\Big[
%	r_{_{TP}}(W) + \frac{[(2M-1)!!]^2}{2^{2M}(2M+1)!}K^{2M}r_{_{TP}}^{2M+1}(W) 
%	+  \mathcal{O}(K^{2M+2}r_{_{TP}}^{2M+3}(W) )  
%	\Big], 	\label{phy1:TP} 
%	\end{align}	
%	
%	
%	\item For spurious modes where $M = 2$
%	\begin{subequations}
%		\label{stp2}
%		\begin{align}
%		\displaystyle
%		k^{\text{TP}}_{\text{FD},s_1}
%		&= k^{ex}
%		\Big[
%		\frac{2i}{K}\text{arcsinh}(\sqrt{6})
%		-\frac{r_{_{TP}}(W)}{2\sqrt{7}} 
%		+ \sqrt{\frac{3}{14}}\cdot \frac{9i}{112}Kr_{_{TP}}^2(W) 
%		+ \frac{45K^2}{1568\sqrt{7}}r_{_{TP}}^3(W)     \notag \\
%		& \hspace{ 1.2 cm } - \frac{5685}{702464}\sqrt{\frac{3}{14}}iK^3r_{_{TP}}^4(W)  
%		+  \mathcal{O}(K^4r_{_{TP}}^5(W))  
%		\Big],    \label{stp1} \\
%		%
%		k^{\text{TP}}_{\text{FD},s_2}
%		&= \overline{	k^{\text{TP}}_{\text{FD},s_1}}.  	
%		\end{align}
%	\end{subequations}
%	\textbf{Note:} To find the general (explicit) form of spurious modes for $M >2$ is quite difficult.
%\end{itemize}
%
%\noindent
%
%\noindent Using the relationship $\displaystyle K = \frac{1}{v}\sqrt{\frac
%	{\epsilon(\hat{\omega};\textbf{p})}{\epsilon_\infty}}W$, we can treated physical solutions \eqref{phy1:TP} and spurious solutions \eqref{stp2}  as a function of $W$ as
%\begin{itemize}
%	\item For physical modes
%	\begin{align}
%	\displaystyle k^{\text{TP}}_{\text{FD},p}
%	= 
%	\begin{cases}
%	\displaystyle k^{ex}
%	\left(
%	1 + 
%	\frac{1}{12}\left( \frac{\delta(\hat{\omega};\textbf{p})}{\epsilon(\hat{\omega};\textbf{p})} +1 + \frac{\epsilon(\hat{\omega}:\textbf{p})}{2\epsilon_\infty\nu^2}\right)W^2
%	+ \mathcal{O}(W^4)
%	\right)  &; M = 1, \\ \\
%	% 
%	\displaystyle
%	k^{ex}
%	\Big(
%	r_{_{TP}}(W)
%	+ \frac{[(2M-1)!!]^2}{2^{2M}(2M+1)!}\left( \frac{\epsilon(\WH{\omega};\textbf{p})}{\epsilon_\infty \nu^2} \right)^M W^{2M}
%	+  \mathcal{O}(W^{2M+2})  
%	\Big)  &; M \geq 2. 
%	\end{cases}    \label{pptp1}
%	\end{align}
%	\item For spurious modes $M = 2$
%	\begin{align}
%	\displaystyle
%	k^{\text{TP}}_{\text{FD},s_1}
%	&= k^{ex}
%	\Big[
%	\sqrt{\frac{\epsilon_\infty}{\epsilon(\hat{\omega};\textbf{p})}}\frac{2\nu i}{W}\text{arcsinh}(\sqrt{6})
%	+ 
%	\left( -\frac{1}{2\sqrt{7}} + \frac{9i}{112\nu}\sqrt{\frac{3\epsilon(\hat{\omega};\textbf{p})}{14\epsilon_\infty}} \right)W
%	+  \mathcal{O}(W^2)  
%	\Big],  \label{sstp1}\\
%	%
%	k^{\text{TP}}_{\text{FD},s_2} 
%	&= \overline{	k^{\text{TP}}_{\text{FD},s_1}}. \label{sstp2}
%	\end{align}
%\end{itemize} 
%
%
%
%
%For $W \rightarrow 0$, we see that $r(W) \rightarrow 1$. It proves to be that both physical (equation \eqref{pplf1} and \eqref{pptp1}) and spurious (equations \eqref{sslf1}-\eqref{sslf2} and \eqref{sstp1}-\eqref{sstp2}) modes converge to the physical and spurious modes of the FD4M scheme. 
%
%To analyze the behavior of the physical solutions of the higher order scheme reducing the dispersion error, we first consider the relative phase error in equation \eqref{pplf1} as
%\begin{align}
%\displaystyle 
%\frac{k^{\text{LF}}_{\text{FD},p} - \displaystyle k^{ex}}{\displaystyle k^{ex}}
%= 
%\begin{cases}
%\displaystyle
%\frac{1}{12}\left( \frac{\delta(\hat{\omega};\textbf{p})}{\epsilon(\hat{\omega};\textbf{p})} - \frac{1}{2} + \frac{\epsilon(\hat{\omega}:\textbf{p})}{2\epsilon_\infty\nu^2}\right)W^2
%+ \mathcal{O}(W^4)
%  &; M = 1, \\ \\
%  \displaystyle
%\frac{1}{12}\left( \frac{\delta(\hat{\omega};\textbf{p})}{\epsilon(\hat{\omega};\textbf{p})} - \frac{1}{2} \right)W^2 
%+ \frac{[(2M-1)!!]^2}{2^{2M}(2M+1)!}\left( \frac{\epsilon(\WH{\omega};\textbf{p})}{\epsilon_\infty \nu^2} \right)^M W^{2M}
%+  \mathcal{O}(W^{2M+2})  
%  &; M \geq 2.  \label{sp1}
%\end{cases}  
%\end{align}
%
%\noindent Note that in the second order scheme (i.e. $M=1$), the CFL number is $\nu/\nu_{\text{max}}=0.7$, i.e. $\nu = 0.7$.
%  The relative phase error of higher order reduces the dispersion error if it satisfies the  condition
%\begin{align}
%\displaystyle
%\left| \frac{\epsilon(\hat{\omega}:\textbf{p})}{24\epsilon_\infty\nu^2} \right|^2
%+ \frac{1}{288\epsilon_\infty \nu^2}
%\left[
%\overline{\left( \frac{\delta(\hat{\omega};\textbf{p})}{\epsilon(\hat{\omega};\textbf{p})} - \frac{1}{2} \right) } \epsilon(\hat{\omega}:\textbf{p})
%+ 
%\left( \frac{\delta(\hat{\omega};\textbf{p})}{\epsilon(\hat{\omega};\textbf{p})} - \frac{1}{2} \right) \overline{ \epsilon(\hat{\omega}:\textbf{p}) }
%\right]
%\geq 0,
%\label{sp3}
%\end{align}
%
%\noindent where the absolute and the bar notation are the modulus and the complex conjugate, respectively. For the simple case $\WH{\gamma} = 0$, the condition \eqref{sp3} is 
%\begin{align}
%\displaystyle
%\frac{\displaystyle\left(\frac{\epsilon_d}{\epsilon_\infty}\right)^2
%	+ (1-2\nu^2)(\WH{\omega}^2 - 1)^2
%	- 2 \left(\frac{\epsilon_d}{\epsilon_\infty}\right)\left(\WH{\omega}^2-1 + \nu^2(1-3\WH{\omega}^2)\right)}{576\nu^4(\WH{\omega}^2-1)^2}
%\geq 0. \label{sp33}
%\end{align}
%
%
%To analyze the condition \eqref{sp33}, for $0 < \nu < 1/\sqrt{2}$ and $0\leq \WH{\omega} < 1$, then the condition \eqref{sp33} holds, see Figure \ref{Fig:sp}. This means that  the leading term of the discrete (2,2) leapfrog scheme and the discrete $(2,2M)$ leap-frog scheme satisfy the condition \eqref{sp33} so that the dispersion error of the discrete $(2,2)$ leap-frog scheme is higher than the discrete $(2,2M)$ leap-frog scheme, see the left plot in Figure \ref{Fig:sp}. 
%
%
%However, in the different material, the condition \eqref{sp33} depends on $\epsilon_d/\epsilon_\infty, \nu$ and $\WH{\omega}$ so one needs to choose optimal parameters carefully to imply the reduction of higher order scheme over the second scheme. For example if $1/\sqrt{2} < \nu < 1$ and $\epsilon_d/\epsilon_s \in (0,2\nu^2-1)$, the condition \eqref{sp33} becomes
%\begin{align}
%\displaystyle
%\label{sp33_2}
%-\frac{2\nu^2-1}{576\nu^4(\WH{\omega}^2-1)^2} 
%\left[ \WH{\omega}^2 -q + p \right]
%\left[ \WH{\omega}^2 -q - p\right].
%\end{align}    
%
%\noindent where 
%\begin{align} \label {cond1} 
%\displaystyle 
%	p = \frac{\nu}{2\nu^2-1} 
%	\sqrt{  \frac{\epsilon_d}{\epsilon_{\infty}}
%	\left[ 4(2\nu^2-1) + \frac{\epsilon_d}{\epsilon_{\infty}}(9\nu^2-4)  \right]
%    } 
%	;\qquad
%	\displaystyle
%	q = \frac{1}{2\nu^2-1} \left[
%	(2\nu^2-1) + \frac{\epsilon_d}{\epsilon_{\infty}}(3\nu^2-1)
%	\right].
%\end{align}
%
%
%\noindent Based on such assumptions, we see that both $p$ and $q$ are positive and also satisfy $\displaystyle p+q > \frac{\epsilon_d}{\epsilon_{\infty}}$ and $q-p>1$. So the condition to guarantee that the dispersion error of discrete (2,2) leapfrog scheme is higher that the discrete $(2,2M)$ scheme is 
%\begin{align}
%\displaystyle
%\label{cond2}
%\sqrt{q-p} \leq \WH{\omega} 
%\leq \sqrt{q+p}.
%\end{align}  
%
%\noindent The region outside the domain \eqref{cond2} shows that the discrete (2,2) scheme has less dispersion error than discrete $(2,2M)$ scheme whose the explicit form is given as equation \eqref{eq:region}. To compare between $2M$ and $2(M+1)$ order schemes, we can do the same analysis by comparing the leading term $W^{2M}$ to find the condition to conclude that the higher scheme reduce the dispersion error.
%
%For $\WH{\gamma} = 0.01$, the condition \eqref{sp3} is positive except for the region around $\WH{\omega} = \sqrt{\epsilon_s/\epsilon_\infty}$. This analysis confirms in Figure \ref{Fig:Phase_Error_FD_fully1} and also the four physical quantities in Figure \ref{Fig:phy_FD1}-\ref{Fig:FD_TP_phy} that higher order schemes reduce the dispersion error over lower order scheme on the region outside $\WH{\omega} = \sqrt{\epsilon_s/\epsilon_\infty}$. Similarly, $2(M+1)$ order schemes provide lower dispersion error than $2M$ order scheme. The condition \eqref{sp3} depends on  $\WH{\gamma}$ besides $\epsilon_d/\epsilon_\infty, \nu$ and $\WH{\omega}$. For the case of higher $\WH{\gamma}$ with fixed parameters $\epsilon_s,\epsilon_\infty$ and $\nu$, the condition \eqref{sp3} will be changed, see Figure \ref{Fig:coeff}.  
%
%
%\begin{figure}[H]
%	\centering
%	\includegraphics[scale=0.55]{pics/gm0}
%		\includegraphics[scale=0.55]{pics/gm01}
%	\caption{The condition \eqref{sp3} and \eqref{sp33} for different $\widehat{\gamma}$ between the second order and fourth order scheme for chosen parameters $\epsilon_d/\epsilon_\infty, \nu$. Left: $\widehat{\gamma} = 0$. Right: $\widehat{\gamma} = 0.01$}
%	\label{Fig:sp}
%\end{figure}
%
%
%
%
%
%
%
%
%
%
%However, for the case of spurious modes we see that all spurious modes contain the factor $1/W$, which leads to undesirable results when $\Delta t \rightarrow 0$ (equivalently to $W \rightarrow 0$). In Figure \ref{Fig: Spurious}, we plot the modulus of ratios between spurious solutions and the exact wave number, $\displaystyle \left| k^{*}_{\text{FD},s}/k^{\text{ex}} \right|$ as a function of $W$ for the case $M = 2,3$ and 4. 
%\begin{figure}[H]
%	\centering
%	\includegraphics[scale=0.28]{pics/LF_M2}
%	\includegraphics[scale=0.28]{pics/LF_M3}
%	\includegraphics[scale=0.28]{pics/LF_M4} \\
%	\includegraphics[scale=0.28]{pics/TP_M2}
%	\includegraphics[scale=0.28]{pics/TP_M3}
%	\includegraphics[scale=0.28]{pics/TP_M4} 		
%	\caption{The ratio of $\displaystyle \left| k^{*}_{\text{FD},s}/k^{\text{ex}} \right|$ for $\WH{\gamma} = 0.01$. Top: leap-frog scheme. Bottom: trapezoidal scheme Left: $M = 2$, Center: $M=3$, Right: $M=4$, where small figure represents the ratio of physical mode and the exact wave number.}
%	\label{Fig: Spurious}
%\end{figure}
%
%\noindent We found that both physical and spurious modes behave similarly for $ W\in [0.5,1)$ and are exploded exponentially when $W \rightarrow 1$. However, for $W \rightarrow 0$, the spurious modes behave differently to the physical modes, which supports our previous argument that the spurious contain the factor $1/W$. Unfortunately, it's quite difficult to find the (explicit) general forms of spurious modes when $M \geq 3$ so that we have no much information to compare or analyze the behavior of spurious modes.
%
%
